# Supplementary material for: Graph Integration for Diffusion-Based Manifold Alignment
Source: arXiv:2410.22978 source file (2024-10-30)
Supplement: Supplementary file 1 [file supplemental.tex]

To include:

Comparisons (quantitative and qualitative) using:
  SPUD:
    1) Different aggregation functions
    2) Effects of number of anchors
    3) 

  DIG:
    1) The effects of the choice of t
    2) Inclusion or exclusion of density normalization
    3) Effects of number of anchors

Partial alignment? That is, where we do not have guaranteed matches in each domain.
